# Supplementary material for: How Continuous Symmetry Stabilizes the Ordered Phase of Polar Flocks
Source: arXiv:2602.16865 ancillary file (2026-02-18)
Supplement: Supplementary file 1 [file SM.pdf]

# Supplemental Material for: "How Continuous Symmetry Stabilizes the Ordered Phase of Polar Flocks"

Omer Granek,[1] Hugues Chaté,[2,3,4] Yariv Kafri,[5] Sunghan Ro,[6] Alexandre Solon,[4] and Julien Tailleur[7]

[1]Leinweber Institute for Theoretical Physics & Kadanoff Center for Theoretical Physics, University of Chicago, 933 E 56th St, Chicago, Illinois 60637, USA
[2]Service de Physique de l'Etat Condensé, CEA, CNRS Université Paris-Saclay, CEA-Saclay, 91191 Gif-sur-Yvette, France
[3]Computational Science Research Center, Beijing 100094, China
[4]Sorbonne Université, CNRS, Laboratoire de Physique Théorique de la Matière Condensée, 75005 Paris, France
[5]Department of Physics, Technion – Israel Institute of Technology, Haifa 32000, Israel
[6]Department of Physics, Harvard University, Cambridge, Massachusetts 02138, USA
[7]Department of Physics, Massachusetts Institute of Technology, Cambridge, Massachusetts 02139, USA

(Dated: February 18, 2026)

Throughout the SM, Eqs. (1-17) and Figs. (1-4) refer to the main text, while Eqs. (S1-S66) and Figs. (S1-S5) refer to supplemental material.

## CONTENTS

A. Numerical details 1
1. Microscopic simulations of the active XY model 1
2. Hydrodynamic simulations 1
3. Numerical protocol for each figure 1
4. Numerical protocol for Supplementary Movies 3

B. Liquid-liquid domain wall solutions for Eqs. (2-3) 3

C. Hydrodynamic description of active $O(d)$ models 4
1. Hierarchy of equations for the spherical-moment dynamics 4
2. Closure 5

D. Liquid-liquid domain wall solutions in active $O(d)$ models 6

E. Stability of front solutions in active $O(d)$ models 7
1. The instability criterion 7
2. Evaluation of Eq. (S.61) 8

F. Supplementary figures 8

G. Description of Movies 8

References 9

## A. NUMERICAL DETAILS

### 1. Microscopic simulations of the active XY model

To simulate the active XY model, we implement a discrete-time dynamics with a time step $dt$.

We first update the particle orientations using the Euler–Maruyama scheme:

$$\theta_n(t+dt) = \theta_n(t) + \gamma\beta dt[p_y(\mathbf{r}_n,t)s_{n,x}(t) - p_x(\mathbf{r}_n,t)s_{n,y}(t)] + \sqrt{2\gamma}dW_n(t) \ , \qquad (S.1)$$

where $\mathbf{r}_n$ is the site where particle $n$ is currently located, $\mathbf{p}(\mathbf{r}_n)$ is the polarisation at that site, and the $\{dW_i\}$ are $N$ independent centered Gaussian white noises with variance $dt$.

Then the particle positions evolve as follows. For each particle $n$, we compute the probability $p_i(\mathbf{s}_n) = D(1 + v\mathbf{s}_n \cdot \mathbf{e}_i)dt$ to hop along one of the four lattice vectors $\mathbf{e}_i \in \{\pm\hat{x}, \pm\hat{y}\}$, and the probability $1 - 4Ddt$ of not moving. We then use tower-sampling to update the particle position accordingly.

Based on the convergence test conducted for the range of parameters explored in this study, we used $dt = 3 \times 10^{-2}$ to produce all results shown in the main text.

### 2. Hydrodynamic simulations

Our simulations of the continuous mean-field equations, Eqs.(2-3) with periodic boundary conditions, are done using a semi-spectral algorithm with Euler time-stepping, 3/2 anti-aliasing, and resolution $dx = 1$ and $dt = 0.1$. The Fourier transforms are performed using the MPI-parallelized implementation of the FFTW3 package.

### 3. Numerical protocol for each figure

Fig. 1. We simulate a system of size $L_x \times L_y = 1000 \times 3000$ with density $\rho_0 = 3$. We first evolve the system for a time $t = 2000$ to produce a homogeneous ordered state with an average polarization along $-\hat{x}$. We then introduce a circular droplet of radius $R$, with density $100\rho_0$ and polarization $\hat{x}$. A first simulation is run to estimate the speed $c$ of the droplet. Then, we use the 'sliding-window method' described in Ref. [1] to run a second simulation in which the

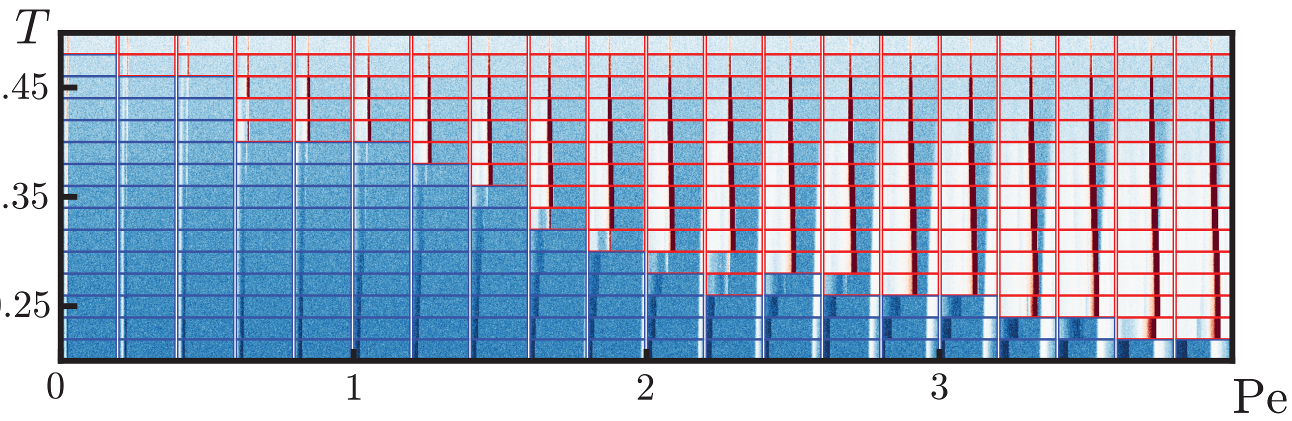


FIG. S1. Array of heatmaps of $m_x$ from a microscopic simulation set of counter-propagating bands. The sampling intervals are 0.2 in Pe and 0.02 in $T$. To facilitate comparisons with Fig. 2, heatmaps corresponding to a stable domain wall, according to the criterion described in Sec. 3, are outlined in red. All others are outlined in blue.

droplet is (roughly) kept at the center of the simulation box by using the measured speed $c$ as a 'sliding speed'. Our high-temperature data at $T = 0.34$ show a small droplet of radius $R = 20$ to grow while the low-temperature data at $T = 0.31$ show a large droplet of radius $R = 60$ to evaporate.

Fig. 2. (Right) To determine the stability of domain walls in microscopic simulations we use the following protocol:

1. On an $L_x \times L_y$ lattice, with $L_x = 6000$ and $L_y = 30$, we place spins randomly to reach an average density $\rho_0 = 60$. All spins are aligned along the $-x$ direction, and the system is evolved for a time $3\gamma^{-1}$ to reach an ordered state with a steady polarization.

2. We then define a rectangular region of size $20 \times L_y$ and flip the particle spins in this region, $\mathbf{s}_n \to -\mathbf{s}_n$, to create a counter-propagating band. To ensure that the band density exceeds that of the surrounding ordered phase, we add additional particles uniformly at random within the band, until its average density is $5\rho_0$. The spins of these additional particles are sampled from a von Mises distribution $P(\mathbf{s}) = e^{\hat{x}\cdot\mathbf{s}/T}/Z$.

3. The simulation is then run for $\Delta t = 3 \times 10^3$. The stability of the domain walls was first checked by visual inspection of the magnetization profiles (see Fig. S1 for an example). To quantitatively discriminate between evaporation and growth of a band, we measure the evolution of $\bar{m}_x(t) = \langle \frac{1}{L_x L_y} \sum_i \mathbf{s}_i(t) \cdot \hat{x} \rangle$. In each simulation, if $\bar{m}_x(t)$ increased by more than $\rho_0/5000$ over the simulation time, we classified the domain wall as stable. For each parameter set, we performed 10 simulations with different random seeds and determined the domain wall stability based on the majority of outcomes. If more runs led to an unstable domain wall, we marked the parameter region as unstable (blue circles). Otherwise, we marked it as stable (red squares).

The symbols corresponding to microscopic simulations are overlayed with a color code, corresponding to the linear stability predicted by the numerical solution of Eq. (7), which we now describe.

1. First, we compute the traveling-front solution $[c, \rho_{\rm f}(z), m_{\rm f}(z)]$ of Eqs. (S.3,S.7) below, by using a shooting method and finding the speed $c$ by bisection to satisfy the boundary conditions (S.2).

2. Second, for this front profile, we solve Eq. (7) for $[r, \lambda(z)]$, using this time a bisection on $r$ to find the heteroclinic trajectory connecting $\lambda(\pm\infty) = \lambda_\pm$.

3. The value of $r$ determines the stability of the domain wall.

The data shown in Fig. 2(c) are consistent with the microscopic numerics and match the analytical stability criterion at small Pe. The domain-wall integration procedure is also used to produce Fig. S2 below.

Fig. 3. The solid lines in panels (a,b,d) are obtained by numerically integrating the domain-wall and linear-stability equations, as described in points 1 & 2 above. Panel (b) compares the resulting profiles with those obtained by direct PDE integration, as described in Sec. 2.

Fig. 4. Left panel: The line $T_c^b$ corresponds to the linear stability of band profiles. Since the problem is invariant in the direction transverse to the order, we use the 1d version of Eqs.(2-3) setting $L_y = 0$. Starting from a counter-propagating band of size $r = 5$ and $\rho_d = 5\rho_0$, we first evolve the system imposing $m_y = 0$ for a time $T_0 = 2000$ so that the initial condition relaxes to a propagating front, as observed in the active Ising model [1]. At $t = T_0$, we add a small perturbation $m_y(T_0) = \varepsilon\xi(x)$ with $\varepsilon = 10^{-10}$ and $\xi(x)$ a Gaussian random field of unit variance. At $T_f = 3000$, if the mean absolute magnetization along $y$ satisfies $\langle|m_y|\rangle > 10^{-8}$, the profile is declared unstable. Other parameters: $v = D = 1$, $L_x = 10000$.

The line $T_c$ is obtained in 2d simulations of Eqs.(2-3). For a given value of $Pe$, it corresponds to the largest $\alpha$ such that a large initial droplet of size $100 \times 1000$ at $\rho_d = 2$ evaporates in a system of size $16384 \times 8192$. A droplet is declared to be evaporating if its magnetization near the center is decreasing at the end of the simulation, when it reaches its tail through the periodic boundary condition. Other parameters: $v = D = 1$.

Right panels. Top: $\alpha = 0.12$, $\gamma = v = D = 1$, size $512 \times 1024$ ($256 \times 614$ shown) with initial droplet of size $12 \times 100$ at $\rho_d = 2$. Bottom: $\alpha = 0.6$, $\gamma = v = D = 1$, size $1024 \times 1024$ ($512 \times 512$ shown) with initial droplet of size $12 \times 200$ at $\rho_d = 2$.

### 4. Numerical protocol for Supplementary Movies

Supplementary Movies 1 & 2: These movies show the simulations used to generate Fig. 1. Supplementary Movie 1 corresponds to Fig. 1(a-c) at $T = 0.34$, with an initial droplet radius of $R = 20$. Supplementary Movie 2 corresponds to Fig. 1(d-f) at $T = 0.31$ and an initial droplet radius of $R = 60$. Further details are provided in Sec. 3.

Supplementary Movies 3 & 4: These movies illustrate how domain-wall stability depends on the model parameters. The initial conditions were prepared by following step 1 and 2 of the Fig. 2 protocol described in Sec. 3. To capture large-scale interface dynamics within a feasible computation time, we used the sliding-window method and tuned parameters. The selected parameters were $L_x = 600$, $L_y = 300$, $\rho_0 = 30$, and $\mathrm{Pe} = 3$. The temperature was $T = 0.3$ for Movie 3 and $T = 0.25$ for Movie 4.

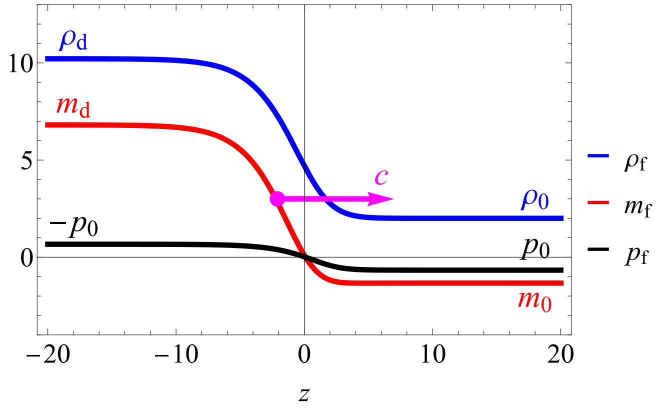


FIG. S2. Domain wall profiles obtained via numeric integration of Eqs. (S.3,S.7) (solid lines) and an illustration of the velocity vector (magenta). Parameters: $v = \gamma = D = 1$, $\rho_0 = 2$ $\beta = 3$).

## B. LIQUID-LIQUID DOMAIN WALL SOLUTIONS FOR EQS. (2-3)

Here, we demonstrate the existence of liquid-liquid domain-wall solutions to Eqs. (2–3), which propagate at a uniquely determined finite speed $c = c(\beta, \mathrm{Pe})$. Our derivation adapts the gradient-expansion approach of the active Ising model [1] to Eqs. (2–3).

We seek a traveling solution for the leading front of an infinite counter-propagating band in the form $[\rho(x,t), \mathbf{m}(x,t)] = [\rho_\mathrm{f}(x-ct), m_\mathrm{f}(x-ct)\hat{\mathbf{x}}]$, where the subscript f denotes a front profile (see Fig. S2.) Introducing $z = x - ct$, such solutions satisfy the boundary conditions

$$\lim_{z\to\pm\infty} \mathbf{p}_\mathrm{f}(z) = \pm p_0 \hat{\mathbf{x}} \quad \text{and} \quad \lim_{z\to\infty} \rho_\mathrm{f}(z) = \rho_0 \ , \tag{S.2}$$

where $\mathbf{p}_\mathrm{f}(z) = \mathbf{m}_\mathrm{f}(z)/\rho_\mathrm{f}(z)$. Below we show that such a solution exists. It is unique and determines the speed $c$, the density $\lim_{z\to-\infty} \rho_\mathrm{f}(z) \equiv \rho_\mathrm{d}$ and the magnetization $\lim_{z\to-\infty} m_f(z) = -\rho_\mathrm{d} p_0 \equiv m_\mathrm{d}$ in the band.

Inserting the domain-wall ansatz, Eq. (2) for the density field gives

$$-c\partial_z \rho_\mathrm{f} = -v\partial_z m_\mathrm{f} + D\partial_z^2 \rho_\mathrm{f} \ . \tag{S.3}$$

Integrating Eq. (S.3) from $z \to -\infty$ to $z \to +\infty$, and using $\lim_{z\to\infty} \rho_\mathrm{f}(z) = \rho_0$ and $\lim_{z\to\infty} m_\mathrm{f}(z) = m_0$, we obtain

$$\rho_\mathrm{f}(z) = \bar{\rho}(m_\mathrm{f}(z)) - \frac{D}{c}\partial_z \rho_\mathrm{f}(z), \tag{S.4}$$

where we have introduced

$$\bar{\rho}(m_\mathrm{f}) \equiv \rho_0 + \frac{v}{c}(m_\mathrm{f} - m_0) \ . \tag{S.5}$$

To leading order in a gradient expansion, we find

$$\rho_\mathrm{f} = \bar{\rho}(m_\mathrm{f}) + \mathcal{O}(\partial_z m_\mathrm{f}) \ , \tag{S.6}$$

and $p_{\rm f} \simeq \bar{p}(m_{\rm f}) \equiv m_{\rm f}/\bar{\rho}(m_{\rm f})$ with $\bar{\rho}(m_{\rm f})$ given by Eq. (S.4).

For the domain wall ansatz, Eq. (3) becomes

$$-c\partial_z m_{\rm f} = -\frac{v}{2}\partial_z \rho_{\rm f} + D\partial_z^2 m_{\rm f} + \gamma F(p_{\rm f}) m_{\rm f} \; . \tag{S.7}$$

Substituting Eq. (S.6) into Eq. (S.7), we obtain

$$D\frac{d^2 m_{\rm f}}{dz^2} = -\Gamma(c)\frac{dm_{\rm f}}{dz} - \frac{dU}{dm_{\rm f}}, \tag{S.8}$$

$$\Gamma(c) \equiv c - \frac{v^2}{2c} \; , \tag{S.9}$$

$$\frac{dU}{dm_{\rm f}} \equiv \gamma F\left[\bar{p}(m_{\rm f})\right] m_{\rm f} \; . \tag{S.10}$$

Equation (S.8) can be interpreted within a Newton-mapping picture using $z$ as a time coordinate, $D > 0$ as a mass, $\Gamma(c)$ as a friction, and $U(m; c)$ as a potential. In this Newton mapping, a domain wall solution corresponds to a heteroclinic trajectory $m_{\rm f}(z)$ connecting the two maxima of $U(m_{\rm f}; c)$, such that $dm_{\rm f}/dz \to 0$ as $z \to \pm\infty$, and obeying the boundary conditions depicted in Fig. S2. Note that, since $\bar{p}(m_{\rm f})$ is asymmetric when $c$ is finite, $U$ is also asymmetric (see Fig. S3), so that any front solution break the PT symmetry $z \to -z$, $m_{\rm f} \to -m_{\rm f}$.

The domain wall speed is constrained by the conservation law for the particle density field $\rho$, which leads to Eq. (S.4). Evaluating the latter at $z \to -\infty$ yields

$$c = v\frac{\Delta m}{\Delta \rho} = v|p_0|\frac{\rho_{\rm d} + \rho_0}{\rho_{\rm d} - \rho_0} \; . \tag{S.11}$$

Thus, a solution with $c > 0$ requires $\rho_{\rm d} > \rho_0$. Moreover, Eq. (S.11) shows that $\rho_{\rm d}/\rho_0$ is determined by $c$ through

$$\frac{\rho_{\rm d}}{\rho_0} = \frac{c + v|p_0|}{c - v|p_0|}. \tag{S.12}$$

This enforces $c > v|p_0|$. The limits $\rho_{\rm d}/\rho_0 \to \infty$ and $\rho_{\rm d}/\rho_0 \to 1^+$ correspond to $c \to v|p_0|^+$ and $c \to \infty$, respectively.

*Existence by continuity in $c$.* We now employ a continuity argument to show that there exists a unique speed $c^* > v|p_0|$ for which a heterocline $m_{\rm f}(z)$ exists.

(i) For $c \to \infty$, $\rho_{\rm f} \to \rho_0$, so $p \to m_{\rm f}/\rho_0$ and $U$ becomes symmetric. Moreover $\Gamma(c) \to \infty$. The dynamics is thus overdamped, and any trajectory that starts at $m_{\rm f} = m_{\rm d}$ undershoots and arrests at $m_{\rm f} = 0$.

(ii) Equations (2-3) lead to $p_0^2 = 2\alpha(1+\alpha)^2 \le 1/2$ [2]. We thus have $v|p_0| < v/\sqrt{2}$. Because $\Gamma(c = v/\sqrt{2}) = 0$, $U(m_{\rm d}) > U(m_0)$, and the dynamics conserve energy, a trajectory starting at $m = m_{\rm d}$ overshoots $m = m_0$ towards $m = -\infty$ for $c = v/\sqrt{2}$.

In summary, the solution overshoots when $c = v/\sqrt{2} > v|p_0|$, and undershoots in the limit $c \to \infty$. By continuity, there must therefore exist $c^* \in (v/\sqrt{2}, \infty)$ such that the trajectory is a heteroclinic orbit connecting $m_{\rm d}$ to $m_0$. Uniqueness follows because the friction coefficient $\Gamma(c)$ increases monotonically with $c$, whereas the asymmetry of $U$ decreases monotonically with $c$. Consequently, the overshoot–undershoot transition is crossed exactly once, fixing a unique value $c^* > v|p_0|$.

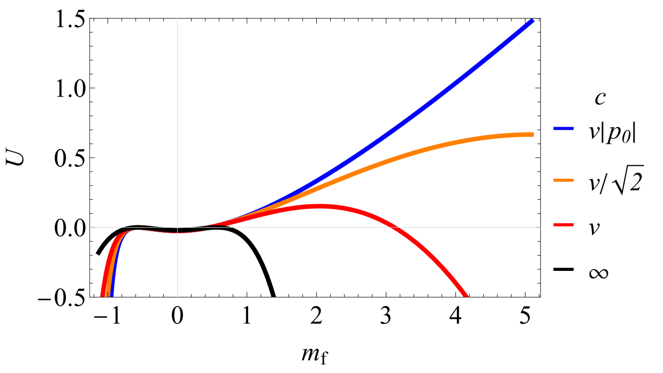


FIG. S3. The inverted potential $U(m_{\rm f}; c)$. The case $c = v|p_0|$ yields an infinite linear ramp, while $c = \infty$ yields a symmetric potential.

## C. HYDRODYNAMIC DESCRIPTION OF ACTIVE $O(d)$ MODELS

In this section, we derive the mean-field hydrodynamic description of active $O(d)$ models. We follow and generalize the derivation of the mean-field hydrodynamic Eqs. (2-3) for the AXYM ($d = 2$) [3] to arbitrary dimension $d$ by projecting the microscopic dynamics onto spherical moments. We then adiabatically eliminate fast modes, and truncate the equation hierarchy to obtain a closed system for $\rho(\mathbf{x}, t)$ and $\mathbf{m}(\mathbf{x}, t)$. We consider a $d$-dimensional lattice $\{\mathbf{r}\}$ with lattice spacing $a$. Particles carry a unit orientation $\mathbf{s} \in S^{d-1}$ and undergo biased hopping from $\mathbf{r}$ to $\mathbf{r} \pm a\hat{\mathbf{e}}_\mu$ at a rate $\frac{D}{a^2} \pm \frac{v}{2a}s_\mu$ with $\mu = 1, \dots, d$. Orientations evolve according to the Stratonovich-Langevin equation,

$$\dot{\mathbf{s}}_i = \gamma\beta(\mathbb{I} - \mathbf{s}_i\mathbf{s}_i)\cdot\mathbf{p}(\mathbf{r}_i) + \sqrt{2\gamma}(\mathbb{I} - \mathbf{s}_i\mathbf{s}_i) \circ \boldsymbol{\eta}_i(t) \; , \tag{S.13}$$

where $\mathbf{p}(\mathbf{r}_i) = \mathbf{m}(\mathbf{r}_i)/\rho(\mathbf{r}_i)$, $\boldsymbol{\eta}_i(t)$ is a Gaussian white noise of unit variance, $\circ$ denotes the Stratonovich product [4], and we use a short-hand notation for the tensor product $\mathbf{s}_i \otimes \mathbf{s}_i \equiv \mathbf{s}_i\mathbf{s}_i$.

### 1. Hierarchy of equations for the spherical-moment dynamics

The mean-field dynamics of the average particle number at site $\mathbf{r}$ with orientation $\mathbf{s}$, denoted $n_{\mathbf{r}} = n(\mathbf{r}, \mathbf{s}, t)$,

reads

$$\partial_t n_{\mathbf{r}} = \sum_{\mu=1}^{d} \left\{ \left( \frac{D}{a^2} + \frac{v s_\mu}{2a} \right) n_{\mathbf{r}-a\hat{\mathbf{e}}_\mu} + \left( \frac{D}{a^2} - \frac{v s_\mu}{2a} \right) n_{\mathbf{r}+a\hat{\mathbf{e}}_\mu} - \frac{2D}{a^2} n_{\mathbf{r}} \right\} - \gamma\beta \nabla_{\mathbf{s}} \cdot \left[ (\mathbb{I} - \mathbf{ss}) \cdot \mathbf{p}_{\mathbf{r}} n_{\mathbf{r}} \right] + \gamma \nabla_{\mathbf{s}}^2 n_{\mathbf{r}} \; , \quad \text{(S.14)}$$

where $\nabla_{\mathbf{s}}$ and $\nabla_{\mathbf{s}}^2$ are the spherical gradient and the spherical Laplacian, respectively.

In the continuum limit, a second-order Taylor expansion leads to

$$n_{\mathbf{r}\pm a\hat{\mathbf{e}}_\mu}(\mathbf{s}) = n_{\mathbf{r}} \pm a\partial_{x_\mu} n_{\mathbf{r}} + \tfrac{a^2}{2}\partial_{x_\mu}^2 n_{\mathbf{r}} + \mathcal{O}(a^3) \; . \quad \text{(S.15)}$$

Inserting this into Eq. (S.14) and summing over $\mu$ gives

$$\partial_t n = -v\mathbf{s}\cdot\nabla n + D\nabla^2 n - \gamma\beta\nabla_{\mathbf{s}}\cdot\Big[(\mathbb{I}-\mathbf{ss})\cdot\mathbf{p}n\Big] + \gamma\nabla_{\mathbf{s}}^2 n. \quad \text{(S.16)}$$

where we rescaled coordinates as $\mathbf{r} \to a\mathbf{r}$ and set $a = 1$.

To derive the hydrodynamic equations, we expand $n(\mathbf{r}, \mathbf{s}, t)$ in irreducible spherical moments [5, 6]:

$$n = \frac{1}{\Omega_d}\rho + \frac{d}{\Omega_d}\mathbf{m}\cdot\mathbf{s} + \frac{d(d+2)}{2\Omega_d}\mathbb{Q} : \left(\mathbf{ss} - \frac{1}{d}\mathbb{I}\right) + \ldots \; , \quad \text{(S.17)}$$

where $\Omega_d = 2\pi^{d/2}\Gamma(d/2)$ is the surface area of a unit sphere and the hydrodynamic modes are the traceless spherical moments,

$$\rho(\mathbf{r}, t) = \int d\Omega(\mathbf{s})\, n(\mathbf{r}, \mathbf{s}, t) \; , \quad \text{(S.18)}$$

$$\mathbf{m}(\mathbf{r}, t) = \int d\Omega(\mathbf{s})\, \mathbf{s}\, n(\mathbf{r}, \mathbf{s}, t) \; , \quad \text{(S.19)}$$

$$\mathbb{Q}(\mathbf{r}, t) = \int d\Omega(\mathbf{s}) \left(\mathbf{ss} - \frac{1}{d}\mathbb{I}\right) n(\mathbf{r}, \mathbf{s}, t) \; . \quad \text{(S.20)}$$

Integrating Eq. (S.16) over $\mathbf{s}$, the angular terms vanish, resulting in the density equation

$$\partial_t \rho = -v\nabla\cdot\mathbf{m} + D\nabla^2\rho \; . \quad \text{(S.21)}$$

To obtain the magnetization equation, we multiply Eq. (S.16) by $s_\mu$ and integrate over $\mathbf{s}$. Integrating the alignment term by parts yields

$$-\int d\Omega(\mathbf{s}) s_\mu \nabla_{\mathbf{s}} \cdot [(\mathbb{I} - \mathbf{ss}) \cdot \mathbf{p}n] = \frac{d-1}{d} m_\mu - \frac{(\mathbb{Q}\cdot\mathbf{m})_\mu}{\rho} \; , \quad \text{(S.22)}$$

where we have used $(\mathbb{I} - \mathbf{ss}) : \mathbf{p}\nabla_{\mathbf{s}} s_\mu = p_\mu - (\mathbf{s}\cdot\mathbf{p}) s_\mu$ and $\mathbf{p} = \mathbf{m}/\rho$. Similarly, using $\nabla_{\mathbf{s}}^2 s_\mu = -(d-1)s_\mu$ and integrating the rotational diffusion term by parts, we find

$$\int d\Omega(\mathbf{s}) s_\mu \nabla_{\mathbf{s}}^2 n = -(d-1) m_\mu \; . \quad \text{(S.23)}$$

We thus obtain

$$\partial_t \mathbf{m} = -v\left(\frac{1}{d}\nabla\rho + \nabla\cdot\mathbb{Q}\right) + D\nabla^2\mathbf{m} + \gamma\beta\left(\frac{d-1}{d}\mathbf{m} - \frac{1}{\rho}\mathbb{Q}\cdot\mathbf{m}\right) - \gamma(d-1)\mathbf{m} \; . \quad \text{(S.24)}$$

For the nematic equation, we use the identity,

$$(\mathbb{I} - \mathbf{ss}) : \mathbf{p}\nabla_{\mathbf{s}}(s_\mu s_\nu) = s_\nu p_\mu + s_\mu p_\nu - 2(\mathbf{s}\cdot\mathbf{p}) s_\mu s_\nu \; . \quad \text{(S.25)}$$

Multiplying Eq. (S.16) by $s_\mu s_\nu - \delta_{\mu\nu}/d$ and integrating by parts then yields

$$\partial_t Q_{\mu\nu} = -v\partial_{x_\sigma}\left(T_{\mu\nu\sigma} - \frac{\delta_{\mu\nu}}{d} m_\sigma\right) + D\nabla^2 Q_{\mu\nu} + \gamma\beta[p_\mu m_\nu + p_\nu m_\mu - 2p_\sigma T_{\mu\nu\sigma}] - 2\gamma d Q_{\mu\nu} \; , \quad \text{(S.26)}$$

where $T_{\mu\nu\sigma} \equiv \int d\Omega(\mathbf{s}) s_\mu s_\nu s_\sigma n$ and we have used

$$\nabla_{\mathbf{s}}^2\left(s_\mu s_\nu - \frac{\delta_{\mu\nu}}{d}\right) = -2d\left(s_\mu s_\nu - \frac{\delta_{\mu\nu}}{d}\right) \; . \quad \text{(S.27)}$$

Neglecting $\nabla\cdot\mathbb{Q}$ in Eq. (S.24) and taking a fast-variable approximation in Eq. (S.27) while neglecting all its gradient terms lead to Eq. (2-3) in the main text. Below, we show that our results are robust to implementing another closure, inspired by [3, 7, 8] and which leads to dynamics akin to the Toner-Tu equations.

### 2. Closure

To close the hierarchy, we follow the standard Boltzmann-Ginzburg-Landau (BGL) approach developed for the Vicsek model [3, 7, 8]. We work deep in the ordered phase, but close to the mean-field transition at $\beta_c = d$, so that the order is small: $\mathbf{p} \sim \epsilon$, where $\beta - d \simeq \epsilon^2$. To order $\epsilon^3$, a closed system of equations can then be obtained by truncating the spherical hierarchy at the nematic order [3, 8]. Following Ref. [8], we assume the BGL scaling

$$\delta\rho \sim \mathbf{p} \sim \nabla \sim \epsilon \; , \quad \text{(S.28)}$$

where $\delta\rho = \rho - \rho_0$. We then note that $\mathbb{Q}$ is a fast dynamical variable that relaxes at a characteristic rate $2\gamma d$, so that $\partial_t Q_{\mu\nu} \simeq 0$ for $t \gg 1/2\gamma d$.

Next, keeping the leading gradient term on the right-hand side of Eq. (S.26) yields

$$2\gamma d Q_{\mu\nu} \simeq -v\partial_{x_\sigma}\left(T_{\mu\nu\sigma} - \frac{\delta_{\mu\nu}}{d} m_\sigma\right) + \gamma\beta[p_\mu m_\nu + p_\nu m_\mu - 2p_\sigma T_{\mu\nu\sigma}] \; . \quad \text{(S.29)}$$

To evaluate $T_{\mu\nu\sigma} \equiv \int d\Omega(\mathbf{s}) s_\mu s_\nu s_\sigma n$, we insert Eq. (S.17) and truncate at the nematic order. The scalar and nematic terms vanish by symmetry, leaving the polar contribution

$$T_{\mu\nu\sigma} \simeq \frac{\delta_{\mu\nu} m_\sigma + \delta_{\mu\sigma} m_\nu + \delta_{\nu\sigma} m_\mu}{d+2} \; . \quad \text{(S.30)}$$

We thus obtain the closure

$$\mathbb{Q} \simeq -\frac{v}{d(d+2)\gamma}\left\{\frac{1}{2}\left[\nabla\mathbf{m}+(\nabla\mathbf{m})^{\mathrm{T}}\right]-\frac{1}{d}\mathbb{I}\nabla\cdot\mathbf{m}\right\} + \frac{\beta}{d+2}\frac{1}{\rho}\left(\mathbf{m}\mathbf{m}-\frac{|\mathbf{m}|^2}{d}\mathbb{I}\right) . \tag{S.31}$$

To recast Eq. (S.24) explicitly in terms of the hydrodynamic fields, we use

$$\nabla\cdot\left[\frac{1}{\rho}\left(\mathbf{m}\mathbf{m}-\frac{|\mathbf{m}|^2}{d}\mathbb{I}\right)\right] \simeq \mathbf{p}\cdot\nabla\mathbf{m}-\frac{2}{d}(\nabla\mathbf{m})\cdot\mathbf{p} \tag{S.32}$$

$$+\mathbf{p}(\nabla\cdot\mathbf{m}) , \tag{S.33}$$

where we use the fact that terms $\propto \nabla\rho$ are higher order in the expansion. Inserting Eqs. (S.31,S.33) into Eq. (S.24), along with Eq. (S.21), we obtain the closed hydrodynamic description,

$$\partial_t\mathbf{m}+\lambda_1\mathbf{p}\cdot\nabla\mathbf{m}+\tilde{\lambda}_2\mathbf{p}(\nabla\cdot\mathbf{m})+2\lambda_3(\nabla\mathbf{m})\cdot\mathbf{p} = -\frac{v}{d}\nabla\rho+D_0\nabla^2\mathbf{m}+D_1\nabla\nabla\cdot\mathbf{m}+\gamma F(|\mathbf{p}|)\mathbf{m} , \tag{S.34}$$

Here,

$$\lambda_1 \equiv \zeta\left(1-\frac{1}{2d}\right),\quad \tilde{\lambda}_2 \equiv \zeta\left(1+\frac{1}{d^2}\right),\quad \lambda_3 \equiv -\zeta\frac{5}{4d}, \tag{S.35}$$

$$\zeta \equiv \frac{\beta v}{d+2},\ D_0 = D+\frac{v^2}{2d(d+2)\gamma},\ D_1 \equiv \frac{d-2}{2d^2(d+2)}\frac{v^2}{\gamma}. \tag{S.36}$$

The alignment dynamics are captured by $F(p) = \alpha\left[1-(p/p_0)^2\right]$, $\alpha = (d-1)(\beta/d-1)$, and $p_0^2 = (d+2)(\beta-d)/\beta^2$ for $T < T_{\mathrm{MF}} = 1/d$.

The case $d=1$, where $\lambda_1+\tilde{\lambda}_2+2\lambda_3 = 0$ and $D_0+D_1 = D$, coincides with the AIM [9, 10].

Note that changing variables $[\rho, \mathbf{m}] \to [\rho, \mathbf{p}]$ using the chain rule,

$$\partial_t\mathbf{p} = \frac{1}{\rho}\partial_t\mathbf{m}-\mathbf{p}\frac{\partial_t\rho}{\rho} , \tag{S.37}$$

with Eqs. (S.21,S.34) leads to

$$\partial_t\mathbf{p}+\lambda_1\mathbf{p}\cdot\nabla\mathbf{p}+\lambda_2(\nabla\cdot\mathbf{p})\mathbf{p}+\lambda_3\nabla|\mathbf{p}|^2 = -\nabla P_1+D_0\nabla^2\mathbf{p}+D_1\nabla\nabla\cdot\mathbf{p}+\gamma F(|\mathbf{p}|)\mathbf{p} , \tag{S.38}$$

where $\lambda_2 \equiv \tilde{\lambda}_2 - v$ and $P_1 = \frac{v}{d}\log\rho$. Equation (S.38) is the Toner-Tu equation [11], truncated at cubic order in $\epsilon$ within the scaling (S.28).

## D. LIQUID-LIQUID DOMAIN WALL SOLUTIONS IN ACTIVE $O(d)$ MODELS

Here, we generalize the derivation of Sec. B to Eqs. (S.21,S.34), which include higher-order gradient, compatible with the BGL scaling, Eq. (S.28). Namely, we seek flat domain wall solutions $[\rho(x,t), \mathbf{m}(x,t)] = [\rho_{\mathrm{f}}(x-ct), m_{\mathrm{f}}(x-ct)\hat{\mathbf{x}}]$, where $\hat{\mathbf{x}} \equiv \hat{\mathbf{e}}_1$, $x \equiv x_1$. Following the path leading to Eqs. (S.3-S.6) now yields

$$\rho_{\mathrm{f}} = \left(1+\frac{D}{c}\partial_z\right)^{-1}\bar{\rho}(m_{\mathrm{f}}) = \bar{\rho}(m_{\mathrm{f}})-\frac{D}{c}\partial_z\bar{\rho}(m_{\mathrm{f}})+\mathcal{O}(\partial_z^2 m_{\mathrm{f}}) = \rho_0+\frac{v}{c}(m_{\mathrm{f}}-m_0)-\frac{vD}{c^2}\partial_z m_{\mathrm{f}}+\mathcal{O}(\partial_z^2 m_{\mathrm{f}}). \tag{S.39}$$

Starting from Eq. (S.34), Eq. (S.7) generalizes to

$$-(c-\zeta\mu p_{\mathrm{f}})\,\partial_z m_{\mathrm{f}} = -\frac{v}{d}\partial_z\rho_{\mathrm{f}}+(D_0+D_1)\partial_z^2 m_{\mathrm{f}}+\gamma F(p_{\mathrm{f}})m_{\mathrm{f}}, \tag{S.40}$$

where

$$\mu \equiv \frac{\lambda_1+\tilde{\lambda}_2+2\lambda_3}{\zeta} = 2-\frac{3}{d}+\frac{1}{d^2} . \tag{S.41}$$

Substituting $\partial_z\rho_{\mathrm{f}} = \frac{v}{c}\partial_z m_{\mathrm{f}} - \frac{vD}{c^2}\partial_z^2 m_{\mathrm{f}} + \mathcal{O}(\partial_z^3)$ from Eq. (S.39) into Eq. (S.40) and truncating at cubic order in $\partial_z$, we obtain

$$K(c)\frac{d^2 m_{\mathrm{f}}}{dz^2} = -\tilde{\Gamma}[\bar{p}(m_{\mathrm{f}}), c]\frac{dm_{\mathrm{f}}}{dz}-\frac{dU}{dm_{\mathrm{f}}}, \tag{S.42}$$

$$K(c) \equiv D_0+D_1+\frac{v^2 D}{c^2 d} , \tag{S.43}$$

$$\tilde{\Gamma}(p,c) \equiv c-\frac{v^2}{cd}-\zeta\mu p , \tag{S.44}$$

which generalizes Eq. (S.42) to Eqs. (S.21,S.34). Equation (S.42) can be interpreted within the Newton-mapping picture with the time coordinate $z$, a mass $K(c) > 0$, a nonlinear friction $\tilde{\Gamma}(p,c)$, and a potential $U(m;c)$. We note that the additional gradient terms do not alter the expression for $U$, which is still given by Eq. (S.10).

*Existence by continuity in $c$.* We now show that there exists a unique speed $c^* > v|p_0|$ for which a heterocline $m_{\mathrm{f}}(z)$ exists.

(i) As in Sec. B, $\lim_{c\to\infty}\tilde{\Gamma}(p,c) \to \infty$. The dynamics is thus overdamped in this limit, and any trajectory that starts at $m_{\mathrm{f}} = m_{\mathrm{d}}$ undershoots and arrests at $m_{\mathrm{f}} = 0$.

(ii) For $c \to v|p_0|^+$, $m_{\mathrm{d}} = -p_0\rho_{\mathrm{d}} \to \infty$ and an asymptotically linear potential ramp emerges in the interval $|m_0| \ll m_{\mathrm{f}} \ll m_{\mathrm{d}}$ (see Fig. S3). Indeed, expanding $\bar{p}(m_{\mathrm{f}}) = m_{\mathrm{f}}/\bar{\rho}(m_{\mathrm{f}})$ using Eq. (S.4) leads to

$$p(m_{\mathrm{f}}; v|p_0|) = |p_0|\left(1+2\frac{m_0}{m_{\mathrm{f}}}\right)+\mathcal{O}(\varepsilon^2) , \tag{S.45}$$

where $\varepsilon \equiv |m_0|/m_{\mathrm{f}}$. With $F(p) = \alpha\left[1-(p/p_0)^2\right]$ and $p_0 < 0$, Eq. (S.45) then yields

$$F\left(\bar{p}(m_{\mathrm{f}})\right) = -\frac{4\alpha m_0}{m_{\mathrm{f}}}+\mathcal{O}(\varepsilon^2) , \tag{S.46}$$

$$-\frac{dU}{dm_{\mathrm{f}}} = -\gamma F\left[\bar{p}(m_{\mathrm{f}})\right]m_{\mathrm{f}} = 4\gamma\alpha m_0\left[1+\mathcal{O}(\varepsilon)\right] . \tag{S.47}$$

Thus, the force is asymptotically constant for large $m_\mathrm{f}$. For the friction, Eq. (S.44) and $p = |p_0| + \mathcal{O}(\varepsilon)$ yield

$$\tilde{\Gamma}\left(\bar{p}(m_\mathrm{f}), v|p_0|\right) = \Gamma_0 + \mathcal{O}(\varepsilon) \ , \tag{S.48}$$

where $\Gamma_0 \equiv \tilde{\Gamma}(-p_0, v|p_0|)$. A direct inspection of Eq. (S.44) using $\zeta = \beta v/(d+2)$ and Eq. (S.41) reveals that $\Gamma_0 < 0$ for all $\beta > d$. On the potential ramp, Eq. (S.42) reduces to the following evolution equation for the velocity $u \equiv dm_\mathrm{f}/dz$:

$$K_0 \frac{du}{dz} = |\Gamma_0| u - s_0 + \mathcal{O}(\varepsilon) \ , \tag{S.49}$$

with $K_0 \equiv K(v|p_0|)$ and $s_0 \equiv 4\gamma\alpha|m_0|$. The solution of Eq. (S.49) is

$$u(z) \simeq \frac{s_0}{|\Gamma_0|} + \left(u(z_\mathrm{i}) - \frac{s_0}{|\Gamma_0|}\right) e^{\frac{|\Gamma_0|}{K_0}(z-z_i)} \ , \tag{S.50}$$

where $z_\mathrm{i}$ is the initial time of entry to the ramp, for which $m_\mathrm{f}(z_\mathrm{i}) \simeq m_\mathrm{d}$ and $u(z_i) \lesssim 0$. Equation (S.50) thus shows that $u(z) < 0$ and that $u(z)$ diverges exponentially as the particle falls along the ramp. Near $m_\mathrm{f} = 0$, the friction coefficient $\tilde{\Gamma}(\bar{p}(m_\mathrm{f}); v|p_0|)$ changes sign and becomes positive. Nonetheless, since the ramp width $m_\mathrm{d} - |m_0|$ diverges as $c \to v|p_0|^+$, the speed at $m_\mathrm{f} = 0$ can be made arbitrarily high by taking $c$ closer to $v|p_0|$. Since the barrier at $m_\mathrm{f} = m_0 < 0$ is of finite height for all $c > v|p_0|$, the trajectory overshoots $m_0$ at an arbitrarily high speed.

In sum, an overshoot is obtained for $c \to v|p_0|^+$, while an undershoot is obtained for $c \to \infty$. By continuity, there exists $c^* \in (v|p_0|, \infty)$ for which the trajectory is a heterocline connecting $m_\mathrm{d}$ and $m_0$.

Uniqueness can be proven by noticing that the friction coefficient $\tilde{\Gamma}(p, c)$ increases monotonically with $c$, while the asymmetry of $U$ and the mass $K(c)$ decrease monotonically with $c$. The overshoot-to-undershoot transition is therefore crossed once, fixing a unique $c^* > v|p_0|$.

## E. STABILITY OF FRONT SOLUTIONS IN ACTIVE $O(d)$ MODELS

Here, we extend the linear stability analysis of the main text to the BGL closure leading to Eqs. (S.21) and (S.34). We consider the linear stability of the liquid-liquid domain-wall solution $[\rho_\mathrm{f}(x-ct), m_\mathrm{f}(x-ct)\hat{\mathbf{x}}]$ to a small transverse perturbation $\delta m_y(x,t)\hat{\mathbf{y}}$ where $\hat{\mathbf{y}} = \mathbf{e}_\mu$, $\mu = 2, ..., d$. We then linearize Eq. (S.34) as

$$[\partial_t + \lambda_1 p_\mathrm{f}(x-ct)\partial_x]\delta m_y(x,t) = D_0\partial_x^2 \delta m_y(x,t) + \gamma F[p_\mathrm{f}(x-ct)]\delta m_y(x,t) \ , \tag{S.51}$$

where $p_\mathrm{f} = m_\mathrm{f}/\rho_\mathrm{f}$. Equation (S.51) generalizes Eq. (5) to the BGL closure. Since $p_\mathrm{f} = p_\mathrm{f}(z)$, with $z = x - ct$, inserting the ansatz $\delta m_y(x,t) = e^{rt} M_y(z)$ into Eq. (S.51) leads to

$$\left[D_0\partial_z^2 + \tilde{c}(z)\partial_z - r\right] M_y = -\gamma F(p_\mathrm{f}) M_y \ , \tag{S.52}$$

$$\tilde{c}(z) \equiv c - \lambda_1 p_\mathrm{f}(z) \ . \tag{S.53}$$

The effect of the BGL closure is thus to promote $c$ in Eq. (6) to $\tilde{c}(z)$ in Eq. (S.52). As we show below, this does not alter the conclusion of the main text: Eq. (S.52) admits a unique solution $[r, M_y(z)]$. The stability transition line $r(\mathrm{Pe}, \alpha) = 0$ is characterized below.

### 1. The instability criterion

To determine the existence and uniqueness of the instabilities, we insert the Cole-Hopf transformation $M_y(z) = \delta m_0 \exp[-\int_0^z dz' \lambda(z')]$ into Eq. (S.52), leading to,

$$D_0 \frac{d\lambda}{dz} = -\partial_\lambda \tilde{V}(\lambda, z) + \gamma F[p_\mathrm{f}(z)] \ , \tag{S.54}$$

$$\tilde{V}(\lambda, z) = r\lambda + \frac{1}{2}\tilde{c}(z)\lambda^2 - \frac{1}{3}D_0\lambda^3 \ , \tag{S.55}$$

where we use the Newton-mapping interpretation of $z$ as a time coordinate and the potential $\tilde{V}$ is depicted in Fig. S4. The effect of the BGL closure on Eq. (7) is thus to promote $V(\lambda) \to \tilde{V}(\lambda, z)$. Like $\tilde{c}(z)$, $\tilde{V}(\lambda, z)$ only varies with $z$ near the domain wall.

At any time $z$, the time-dependent potential $\tilde{V}(\lambda, z)$ has two finite fixed points $\lambda_\pm^0(z)$. Since the driving $\gamma F[p_\mathrm{f}(z)]$ is localized in the vicinity of the domain wall and the dynamics is overamped, a solution $\lambda(z)$ connects one of the two fixed points for $z = -\infty$ to one of two fixed points for $z = \infty$. We denote the fixed points for $z = \pm\infty$ as $\lambda_\pm^0(\pm\infty) = \lambda_\pm$, where $\lambda_\pm$ are given by (see Fig. S4)

$$\lambda_\pm = \frac{c_\pm \pm \sqrt{c_\pm^2 + 4D_0 r}}{2D_0} \ , \tag{S.56}$$

and $c_\pm = \tilde{c}(\pm\infty) = c \mp \lambda_1 p_0$. Therefore, to obtain a solution that satisfies the boundary conditions, we need to take $\lambda(-\infty) = \lambda_-$ and $\lambda(\infty) = \lambda_+$. This implies for $M_y$ the same the far-field behavior as in Eq. (8) of the main text:

$$M_y \sim \begin{cases} e^{-\lambda_- z}, & z \ll -w \\ e^{-\lambda_+ z}, & z \gg w \end{cases} \ , \tag{S.57}$$

Furthermore, the boundary conditions lead to the selection of $r$: given $c$ and $\gamma F[p_\mathrm{f}(z)]$, there exists a unique value of $r$ for which the driving brings the virtual particle from the local minimum at $\lambda = \lambda_-$ to the local maximum at $\lambda = \lambda_+$. Integrating Eq. (S.54) over $z$, we find that this solution satisfies

$$D_0 \Delta\lambda = -\int dz \partial_\lambda \tilde{V}(\lambda, z) + \int dz \gamma F[p_\mathrm{f}(z)], \tag{S.58}$$

where $\Delta\lambda = \lambda(\infty) - \lambda(-\infty)$. For a solution to exist and a force $r > 0$ to be selected, the driving must 1) overcome the potential barrier for $r = 0$ and 2) overshoot $\lambda = \lambda_+$, i.e., $\Delta\lambda|_{r=0} > \Delta\lambda_\pm|_{r=0}$ where $\Delta\lambda_\pm \equiv \lambda_+ - \lambda_-$. Moreover, $\Delta\lambda|_{r=0} = \infty$ if the driving impulse $\int dz\gamma F[p_f(z)]$ exceeds the impulse of the potential force up to the potential maximum $\lambda_+^0(z)|_{r=0} = \tilde{c}(z)/D_0$. Lastly, Eq. (S.56) provides

$$\Delta\lambda|_{r=0} = \frac{c_+ - c_-\Theta(-c_-)}{D_0} = \frac{c_{\max}}{D_0} , \tag{S.59}$$

$$c_{\max} = \begin{cases} c_+ , & c > \lambda_1|p_0| \\ 2\lambda_1|p_0| , & c < \lambda_1|p_0| \end{cases} . \tag{S.60}$$

Therefore, the condition for a solution $[r > 0, \lambda(z)]$ to exist is

$$c_{\max} + \int dz\Theta[\tilde{c}(z)/D_0 - \lambda(z)]\partial_\lambda\tilde{V}(\lambda, z) < \int dz\gamma F[p_f(z)] , \tag{S.61}$$

which generalizes Eq. (9). When Eq. (S.61) is satisfied, the perturbation $\delta m_y$ grows and destroys the domain wall. The stability transition occurs when Eq. (S.61) saturates, i.e. the left-hand side equals the right-hand side.

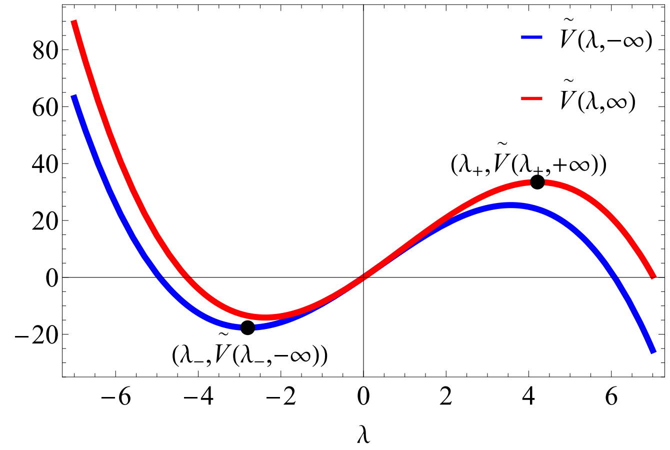


FIG. S4. The potentials $\tilde{V}(\lambda, \pm\infty)$. The fixed points $\lambda_\pm$ are marked in black dots. Left panel: $r = 10$, right panel: $r = 0$. Parameters: $c = 1.3$, $\beta = 2.5$, $D = 1$.

### 2. Evaluation of Eq. (S.61)

To evaluate Eq. (S.61), we use the scaling forms

$$\lambda(z) = \frac{c_{\max}}{D_0}\Lambda\left(\frac{z}{w}\right) , \quad p_f(z) = p_0 P\left(\frac{z}{w}\right) , \tag{S.62}$$

$$\tilde{c}(z) = c_{\max} C\left(\frac{z}{w}\right) , \tag{S.63}$$

where $\Lambda(u)$, $P(u)$, and $C(u)$ are bounded function of Pe and $\alpha$ and $u = z/w$. Inserting Eqs. (S.62)-(S.63) into the left-hand side of Eq. (S.61), we obtain

$$\int dz\Theta(\tilde{c}(z)/D_0 - \lambda)\partial_\lambda\tilde{V} = \frac{c_{\max}^2 w}{D_0} I_{\text{diff}} , \tag{S.64}$$

where

$$I_{\text{diff}} \equiv \int du\left[C(u)\Lambda(u) - \Lambda^2(u)\right]\Theta[C(u) - \Lambda(u)] . \tag{S.65}$$

Substituting Eqs. (S.64) into Eq. (S.61), we finally recover the existence condition, Eq. (10), albeit with $c \to c_{\max}$,

$$\tau_{\text{res}} = \frac{w}{c_{\max}} \quad \text{and} \quad \tau_{\text{diff}} = \frac{D_0}{c_{\max}^2 I_{\text{diff}}} = \frac{\xi^2}{D_0 I_{\text{diff}}} , \tag{S.66}$$

where $\xi \equiv D_0/c_{\max}$ amounts to the screening length associated with the transition from diffusion on small scales to advection on large ones [12].

In the limit $\alpha, \text{Pe} \ll 1$ with $\chi \equiv 2\text{Pe}/\alpha d = \mathcal{O}(1)$, Eq. (S.54) reduces to Eq. (14). As shown in the main text, $[\chi, \Lambda(u)] = [4, (1 + \tanh u)/2]$ is its unique solution. Using $\chi \equiv 2\text{Pe}/\alpha d$, we conclude that for $\alpha \ll 1$, the transition line converges to $\text{Pe} = 2d\alpha$, or, equivalently, Eq. (17). The transition line corresponds to the heteroclinic solution $\Lambda(u) = (1 + \tanh u)/2$. Using Eq. (S.62) and $c_{\max} \simeq c$, we recover Eq. (16) for the BGL closure.

In conclusion, up to $c \to c_{\max}$ and the definitions in Eq. (S.66), the stability criterion derived in the main text extends directly to the BGL closure.

## F. SUPPLEMENTARY FIGURES

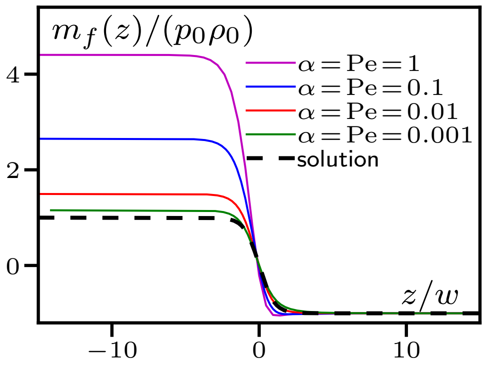


FIG. S5. Rescaled front profile $m_f(z)$ obtained in numerical integration of Eqs. (2-3) with $m_y = 0$ showing the convergence to the analytical solution Eq. (4) with $w = (2D/\gamma\alpha)^{1/2}$. $D = v = 1$.

.

## G. DESCRIPTION OF MOVIES

In this section we briefly describe the supplementary movies. The details of the numerics are given Sec. A4.

- Movie 1 shows an initially small droplet that grows and becomes stable at long times. The movie is terminated when the size of the droplet becomes comparable to the system height.
- Movie 2 shows an initial droplet, larger than the one appearing in Movie 1, that develops an instability at the front and evaporates at long times.
- Movie 3 shows an initial band spanning the full system width that propagates and grows steadily.
- Movie 4 shows an initial band spanning the full system width that becomes unstable due to the growth of a transverse magnetization $m_y$.
- Movie 5-7: Droplet propagation in the hydrodynamic equations. Movie 6 and 7 correspond respectively to the red triangle ($T = 0.3125$) and the green star ($T = 0.44$) shown in Fig. 4, which feature unstable droplets. Movie 5 shows a stable propagating droplet at higher $T = 0.485$. Other parameters: $\gamma = v = D = 1$.

[1] B. Benvegnen, O. Granek, S. Ro, R. Yaacoby, H. Chaté, Y. Kafri, D. Mukamel, A. Solon, and J. Tailleur, Phys. Rev. Lett. **131**, 218301 (2023).
[2] Larger values of $|p_0|$ requires another closure of the mean-field dynamics.
[3] A. Solon, H. Chaté, J. Toner, and J. Tailleur, Phys. Rev. Lett. **128**, 208004 (2022).
[4] In Itō prescription, keeping the norm of $\mathbf{s}_i$ constant would require an extra drift term.
[5] M. E. Cates and J. Tailleur, EPL **101**, 20010 (2013).
[6] A. P. Solon, M. E. Cates, and J. Tailleur, Eur. Phys. J. Spec. Top. **224**, 1231 (2015).
[7] E. Bertin, M. Droz, and G. Grégoire, Phys. Rev. E **74**, 022101 (2006).
[8] A. Peshkov, E. Bertin, F. Ginelli, and H. Chaté, Eur. Phys. J. Spec. Top. **223**, 1315 (2014).
[9] A. P. Solon and J. Tailleur, Phys. Rev. Lett. **111**, 078101 (2013).
[10] A. P. Solon and J. Tailleur, Phys. Rev. E **92**, 042119 (2015).
[11] J. Toner, Phys. Rev. E **86**, 031918 (2012).
[12] T. Sadhu, S. N. Majumdar, and D. Mukamel, Phys. Rev. E **84**, 051136 (2011).
